# Supplementary material for: ReTR: Modeling Rendering Via Transformer for Generalizable Neural Surface Reconstruction
Source: arXiv:2305.18832 source file (2023-11-02)
Supplement: Supplementary file 1 [file appendix.tex]

\section*{Appendix}   

\section{Implementation Details}

\subsection{Experimental Environment} 
Software and hardware environment:
\begin{itemize}
    \item CUDA version: 11.1
    \item cuDNN version: 8.0.5
    \item PyTorch version: 1.10.1
    \item GPU: Nvidia RTX 3090
    \item CPU: Intel Xeon Platinum 8180 @ 2.50 GHz $\times$ 2
\end{itemize}

\subsection{Training Detail} 
Our model is implemented in PyTorch using the PyTorch Lightning framework. During the training stage, we resize the input image to 640 x 512 and the source views to $N=4$. To train our model, we employ the Adam optimizer on a single Nvidia 3090 GPU. Initially, the learning rate is set to $10^{-4}$ and gradually decays to $10^{-6}$ using a cosine learning rate scheduler. Throughout the training, we use a batch size of 2 and set the number of rays to 1024.
To enhance the sampling strategy, we apply a coarse-to-fine approach with both $N_{coarse}$ and $N_{fine}$ set to 64. The $N_{coarse}$ points are uniformly sampled between the near and far plane, while the $N_{fine}$ points are sampled using importance sampling based on the coarse probability estimation.
Regarding the global feature volume $f^{v}$, we set its resolution to K=128. For inference on DTU, the image resolution is set to 800 x 600. For datasets such as BlendedMVS~\cite{yao2020blendedmvs}, ETH3D~\cite{schops2017multi}, and Tanks \& Temples~\cite{Knapitsch2017}, we maintain the original image resolution.
Training our model requires approximately 3 days on a single Nvidia 3090 GPU. Moreover, when constructing larger models such as the large and xlarge models by stacking more layers, the training time will naturally increase due to the increased model size.

\subsection{Mesh and Point Cloud Generation} 
Following the settings employed in VolRecon~\cite{ren2022volrecon}, we generate depth maps from virtual viewpoints by shifting the original camera along its $x$-axis by $d=25$ mm. Subsequently, we perform TSDF fusion and applied the Marching Cubes algorithm to merge all the rendered depths into a voxel grid with a resolution of 1.5 mm and extract a mesh representation.
For point cloud generation, we initially generate 49 depth maps by leveraging the four nearest source views. These 49 depth maps are then fused together to form a unified point cloud.

\section{Technical Details and Discussion}
\begin{wrapfigure}{h}{0.60\linewidth}
\begin{center}
\setlength{\abovecaptionskip}{0.cm}
\vspace{-0.6cm}  
\centerline{\includegraphics[width=0.6\textwidth]{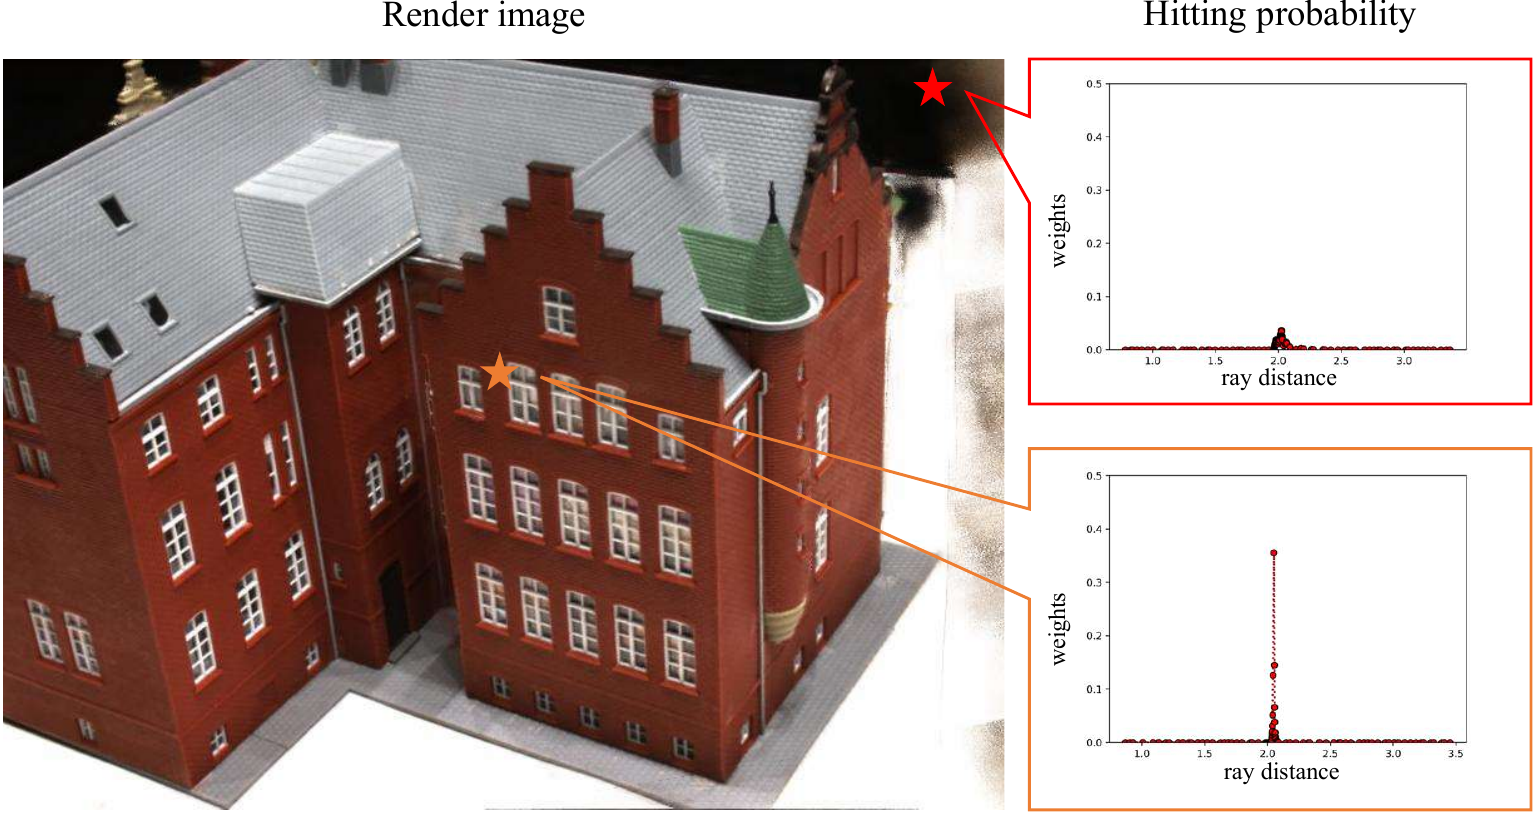}}
% \vspace{0.1cm}  
\caption{Hitting probability comparison.}
\label{fig:discuss_hp}
\vspace{-1cm}  
\end{center}
\end{wrapfigure}

\subsection{Discussion of Hitting Probability} 
The attention score in ReTR can be interpreted as the probability of a ray being \textit{hit}. However, when using \textit{softmax}, the attention scores for each ray are forced to sum up to 1, implying that every ray should be considered a \textit{hit}. To gain further insights, we examine the distribution of attention scores for rays that are \textit{not hitting}. Figure~\ref{fig:discuss_hp} illustrates the results, demonstrating that the transformer intelligently employs a wider distribution to model rays that do \textit{not hit}. The underlying rationale is that the transformer treats the surrounding air as a medium that contributes to the color. When a ray does \textit{not hit}, the transformer aggregates information from the surrounding air to obtain the color from these mediums.

\subsection{Hierarchical Volume Sampling through Attention Map} 
Given that our framework does not incorporate weights as seen in traditional frameworks like NeRF or NueS, we refine the original hierarchical sampling strategy by substituting the weights with the attention scores of each point. This approach, as discussed in the main text, is both straightforward and impactful. Additionally, we highlight that our method exhibits greater robustness in terms of the number of sampling points compared to the current state-of-the-art techniques, thereby offering an additional advantage within our framework.

\subsection{Continous Positional Encoding Proof} 
To imbue our system with positional awareness of actual distance. we initially derive the formula for the attention score, denotes as $s$ of features in $\Mat{x}_i$ and $\Mat{x}_j$:
\begin{equation}
\label{eq:attn_score}
    s = (\mathbf{f}^{f}_i+\mathbf{p}_i)W_qW_k^\top(\mathbf{f}^{f}_j+\mathbf{p}_j)^\top,
\end{equation}
where $\mathbf{p}$ represents the positional encoding in $\Mat{x}$. We subsequently expand Eq.~\eqref{eq:attn_score} as follows:
\begin{equation}
\label{eq:attn_score_2}
    s = (\mathbf{f}^{f}_i)W_qW_k^\top(\mathbf{f}^{f}_j)^\top+(\mathbf{f}^{f}_i)W_qW_k^\top(\mathbf{p}_j)^\top+(\mathbf{p}_i)W_qW_k^\top(\mathbf{f}^{f}_j)^\top+(\mathbf{p}_i)W_qW_k^\top(\mathbf{p}_j)^\top,
\end{equation}
where the fourth component of Eq.\eqref{eq:attn_score_2} denotes the interaction between two locations, and $W_qW_k^\top$ represents the trainable parameters. To ensure our MLP actual positional awareness, we need to make the function satisfy the following conditions:
\begin{equation}
\label{eq:condition}
    (\mathbf{p}_i)(\mathbf{p}_j)^\top = f(t_j-t_i),
\end{equation}
where $t_j-t_i$ denotes the distance between $\Mat{x}_i$ and $\Mat{x}_j$. When we apply our positional encoding (PE), the fourth component of Eq.\eqref{eq:attn_score_2} can be simplified as:
\begin{equation}
\begin{split}
\label{eq:attn_score_3}
    (\mathbf{p}_i)(\mathbf{p}_j)^\top = &\quad [sin(\beta t_i / 10000^{2i/D}),cos(\beta t_i / 10000^{2i/D})] \\
    & \times [sin(\beta t_j / 10000^{2i/D}),cos(\beta t_j / 10000^{2i/D})]^\top,
\end{split}
\end{equation}
\begin{equation}
\begin{split}
\label{eq:attn_score_4}
    (\mathbf{p}_i)(\mathbf{p}_j)^\top = &\quad sin(\beta t_i / 10000^{2i/D})sin(\beta t_i / 10000^{2i/D}) \\
    & +cos(\beta t_j / 10000^{2i/D})cos(\beta t_j / 10000^{2i/D}).
\end{split}
\end{equation}
By applying the sum-to-product identities, we obtain:
\begin{equation}
\label{eq:attn_score_4}
    (\mathbf{p}_i)(\mathbf{p}_j)^\top = cos(\beta (t_j-t_i) / 10000^{2i/D}),
\end{equation}
where $(t_j-t_i)$ represents the actual distance between $\Mat{x}_i$ and $\Mat{x}_j$. Thus, continuous positional encoding enables the attainment of actual positional awareness.

\section{Additional Experimental Results} 
Here we show additional experiment results:
\begin{table}[]
\centering
\resizebox{\textwidth}{!}{%
\begin{tabular}{@{}cccccccccccccccc@{}}
\toprule
\multicolumn{1}{l}{Sample Points} &
  \multicolumn{1}{l}{scan 24} &
  \multicolumn{1}{l}{scan 37} &
  \multicolumn{1}{l}{scan 40} &
  \multicolumn{1}{l}{scan 55} &
  \multicolumn{1}{l}{scan 63} &
  \multicolumn{1}{l}{scan 65} &
  \multicolumn{1}{l}{scan 69} &
  \multicolumn{1}{l}{scan 83} &
  \multicolumn{1}{l}{scan 97} &
  \multicolumn{1}{l}{scan 105} &
  \multicolumn{1}{l}{scan 106} &
  \multicolumn{1}{l}{scan 110} &
  \multicolumn{1}{l}{scan 114} &
  \multicolumn{1}{l}{scan 118} &
  \multicolumn{1}{l}{scan 122} \\ \midrule
16+16 & 1.09 & 2.49 & 1.51 & 1.09 & 1.62 & 1.64 & 0.97 & 1.35 & 1.43 & 1.05 & 1.21 & 0.77 & 0.72 & 1.27 & 1.28 \\
32+32 & 1.06 & 2.30 & 1.46 & 0.97 & 1.35 & 1.53 & 0.89 & 1.38 & 1.34 & 0.92 & 1.10 & 0.74 & 0.60 & 1.10 & 1.17 \\
64+0  & 1.11 & 2.39 & 1.43 & 1.06 & 1.36 & 1.62 & 0.94 & 1.28 & 1.31 & 0.91 & 1.12 & 0.78 & 0.64 & 1.18 & 1.20 \\
128+0 & 1.39 & 2.36 & 1.54 & 1.01 & 1.18 & 1.65 & 0.97 & 1.26 & 1.26 & 0.83 & 1.10 & 0.84 & 0.62 & 1.09 & 1.15 \\ \bottomrule
\end{tabular}%
}
\caption{Chamfer distance of a number of different sampling points, results are shown for each scan under different settings.}
\label{tab:supp_pointnum}
\end{table}

\subsection{Visualization Supplementary} 
Due to space limitations, we provide additional visual results for the experiments in this section. Specifically, we present the results for \textbf{sparse view reconstruction} in Fig.~\ref{fig:sprecon} and \textbf{full view reconstruction} of the point cloud in Fig.~\ref{fig:fullrec}. Furthermore, we include the per-scene results for the number of sampling points in Tab.~\ref{tab:supp_pointnum}.

\subsection{Error Bar of ReTR} 
In order to assess the reproducibility and robustness of our model, we conduct three separate training runs using different random seeds. The corresponding results are presented in Figure~\ref{fig:error_bar}. These results demonstrate that our model exhibits consistent performance across multiple training runs, indicating good reproducibility. Moreover, the minimal variance observes in the results further underscores the robustness of our model.
\subsection{Effectiveness of Stacking Transformer Blocks} 
To explore the potential of simulating more complex light transport effects, we extend our learnable rendering approach by stacking multiple layers of transformer blocks. Specifically, we introduce two variations: \textbf{ReTR-L}, where we stack two transformer blocks, and \textbf{ReTR-XL}, where we stack three transformer blocks. This allows us to experimentally evaluate the effectiveness of a more complex rendering system.
The results of these experiments are summarized in Tab.~\ref{tab:ReTR-BLXL}. The findings indicate that by overlaying multiple layers of transformers, we can simulate complex lighting effects and achieve more powerful results. This demonstrates the potential of our approach to capture intricate light transport phenomena and enhance the overall rendering capabilities.

\subsection{Novel View Synthesis} 
In order to assess ReTR's performance in Novel View Synthesis, a task where many multi-view stereo techniques struggle, we conduct a quantitative comparison with VolRecon~\cite{ren2022volrecon}. The novel views are generated during the full reconstruction for fusing the point clouds as we discussed in the main paper. Our results demonstrate a significant improvement over VolRecon in terms of novel view synthesis, as shown in Tab.~\ref{tab:novel_view_psnr}. Additionally, we provide visualizations of novel view synthesis and depth synthesis in Figure~\ref{fig:synthesis}.
It has been challenging to achieve high-quality results simultaneously in rendering-based studies and reconstruction-based studies, with few methods excelling in both aspects. However, the results achieved by our proposed framework, ReTR, are highly promising, which suggests that a learnable rendering approach based on transformers can effectively integrate both tasks, yielding impressive results on both fronts within a unified framework.

\begin{table}[]
\centering
\resizebox{\textwidth}{!}{%
\begin{tabular}{@{}ccccccccccccccccc@{}}
\toprule
\multicolumn{1}{l}{Models} &
  Mean &
  \multicolumn{1}{l}{scan 24} &
  \multicolumn{1}{l}{scan 37} &
  \multicolumn{1}{l}{scan 40} &
  \multicolumn{1}{l}{scan 55} &
  \multicolumn{1}{l}{scan 63} &
  \multicolumn{1}{l}{scan 65} &
  \multicolumn{1}{l}{scan 69} &
  \multicolumn{1}{l}{scan 83} &
  \multicolumn{1}{l}{scan 97} &
  \multicolumn{1}{l}{scan 105} &
  \multicolumn{1}{l}{scan 106} &
  \multicolumn{1}{l}{scan 110} &
  \multicolumn{1}{l}{scan 114} &
  \multicolumn{1}{l}{scan 118} &
  \multicolumn{1}{l}{scan 122} \\ \midrule
ReTR-B  & \multicolumn{1}{c}{1.17} & 1.05 & 2.31 & 1.44 & 0.98 & 1.18 & 1.52 & 0.88 & 1.35 & 1.30 & 0.87 & 1.07 & 0.77 & 0.59 & 1.05 & 1.12 \\
ReTR-L  & 1.16                     & 0.98 & 2.26 & 1.59 & 1.00 & 1.14 & 1.56 & 0.90 & 1.35 & 1.26 & 0.86 & 1.06 & 0.78 & 0.57 & 1.01 & 1.07 \\
ReTR-XL & 1.15                     & 0.96 & 2.26 & 1.64 & 0.94 & 1.19 & 1.59 & 0.86 & 1.32 & 1.25 & 0.85 & 1.02 & 0.75 & 0.55 & 1.02 & 1.11 \\ \bottomrule
\end{tabular}%
}
\caption{Result of ReTR-Base, ReTR-Large and ReTR-XLarge evaluated on DTU under 3 views setting. We report chamfer distance, the lower the better.}
\label{tab:ReTR-BLXL}
\end{table}

\begin{table}[]
\centering
\resizebox{0.5\textwidth}{!}{%
\begin{tabular}{@{}ccccc@{}}
\toprule
Method   & PSNR$\uparrow$  & MSE$\downarrow$ & SSIM$\uparrow$ & LPIPS$\downarrow$        \\ \midrule
MVSNeRF* & 25.92          & 0.003          & \textbf{0.89} & \textbf{0.19} \\
VolRecon* & 23.37          & 0.004           & 0.80          & 0.30        \\
ReTR-B     & 25.88          & 0.004          & 0.83          & 0.28          \\
ReTR-L    & 26.03          & 0.003          & 0.84          & 0.27          \\
ReTR-XL   & \textbf{26.33} & \textbf{0.003} & 0.84          & 0.27          \\ \bottomrule
\end{tabular}%
}
\caption{Novel View synthesis result on DTU, * denotes our reproduced result.}
\label{tab:novel_view_psnr}
\end{table}

\begin{figure*}[t]
%\vspace{-2em}
\begin{center}
\setlength{\abovecaptionskip}{0.cm}
\centerline{\includegraphics[width=\textwidth]{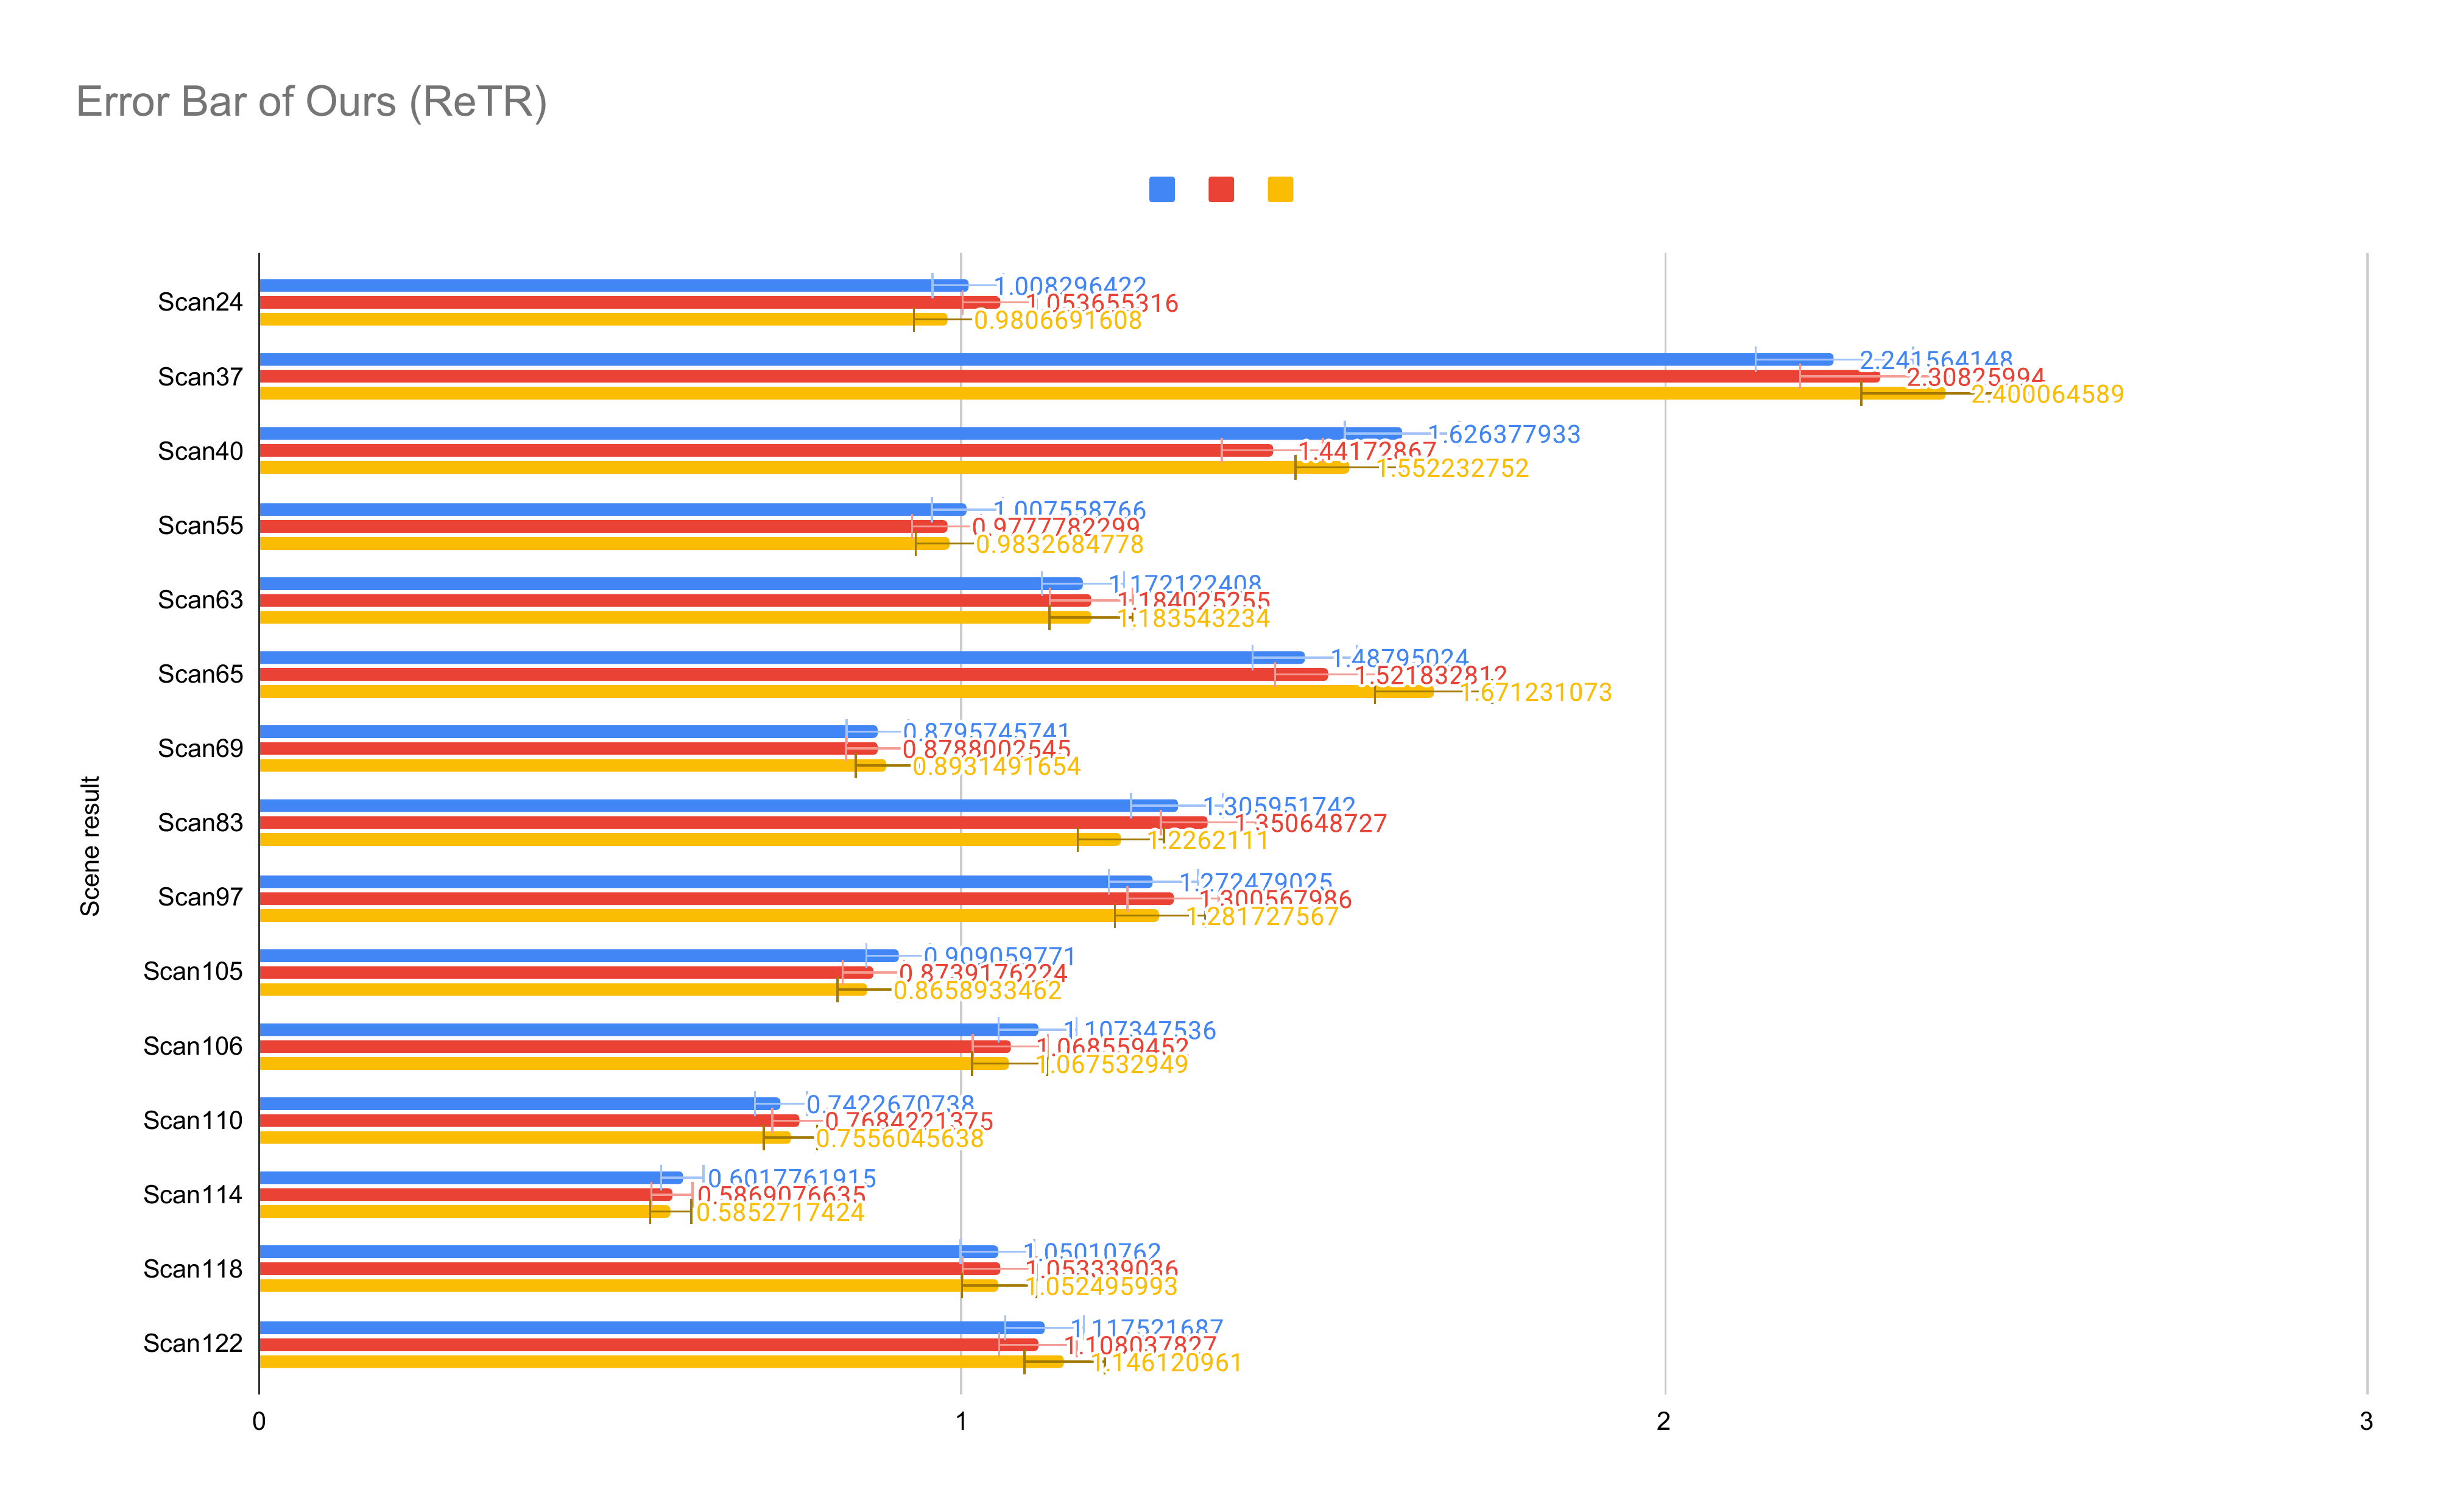}}
% \vspace{0.1cm}  
\caption{Error bar on 3 runs of Ours (ReTR).}
\label{fig:error_bar}
% \vspace{-0.8cm}  
\end{center}
\end{figure*}

\begin{figure*}[t]
%\vspace{-2em}
\begin{center}
\setlength{\abovecaptionskip}{0.cm}
\centerline{\includegraphics[width=1.0\textwidth]{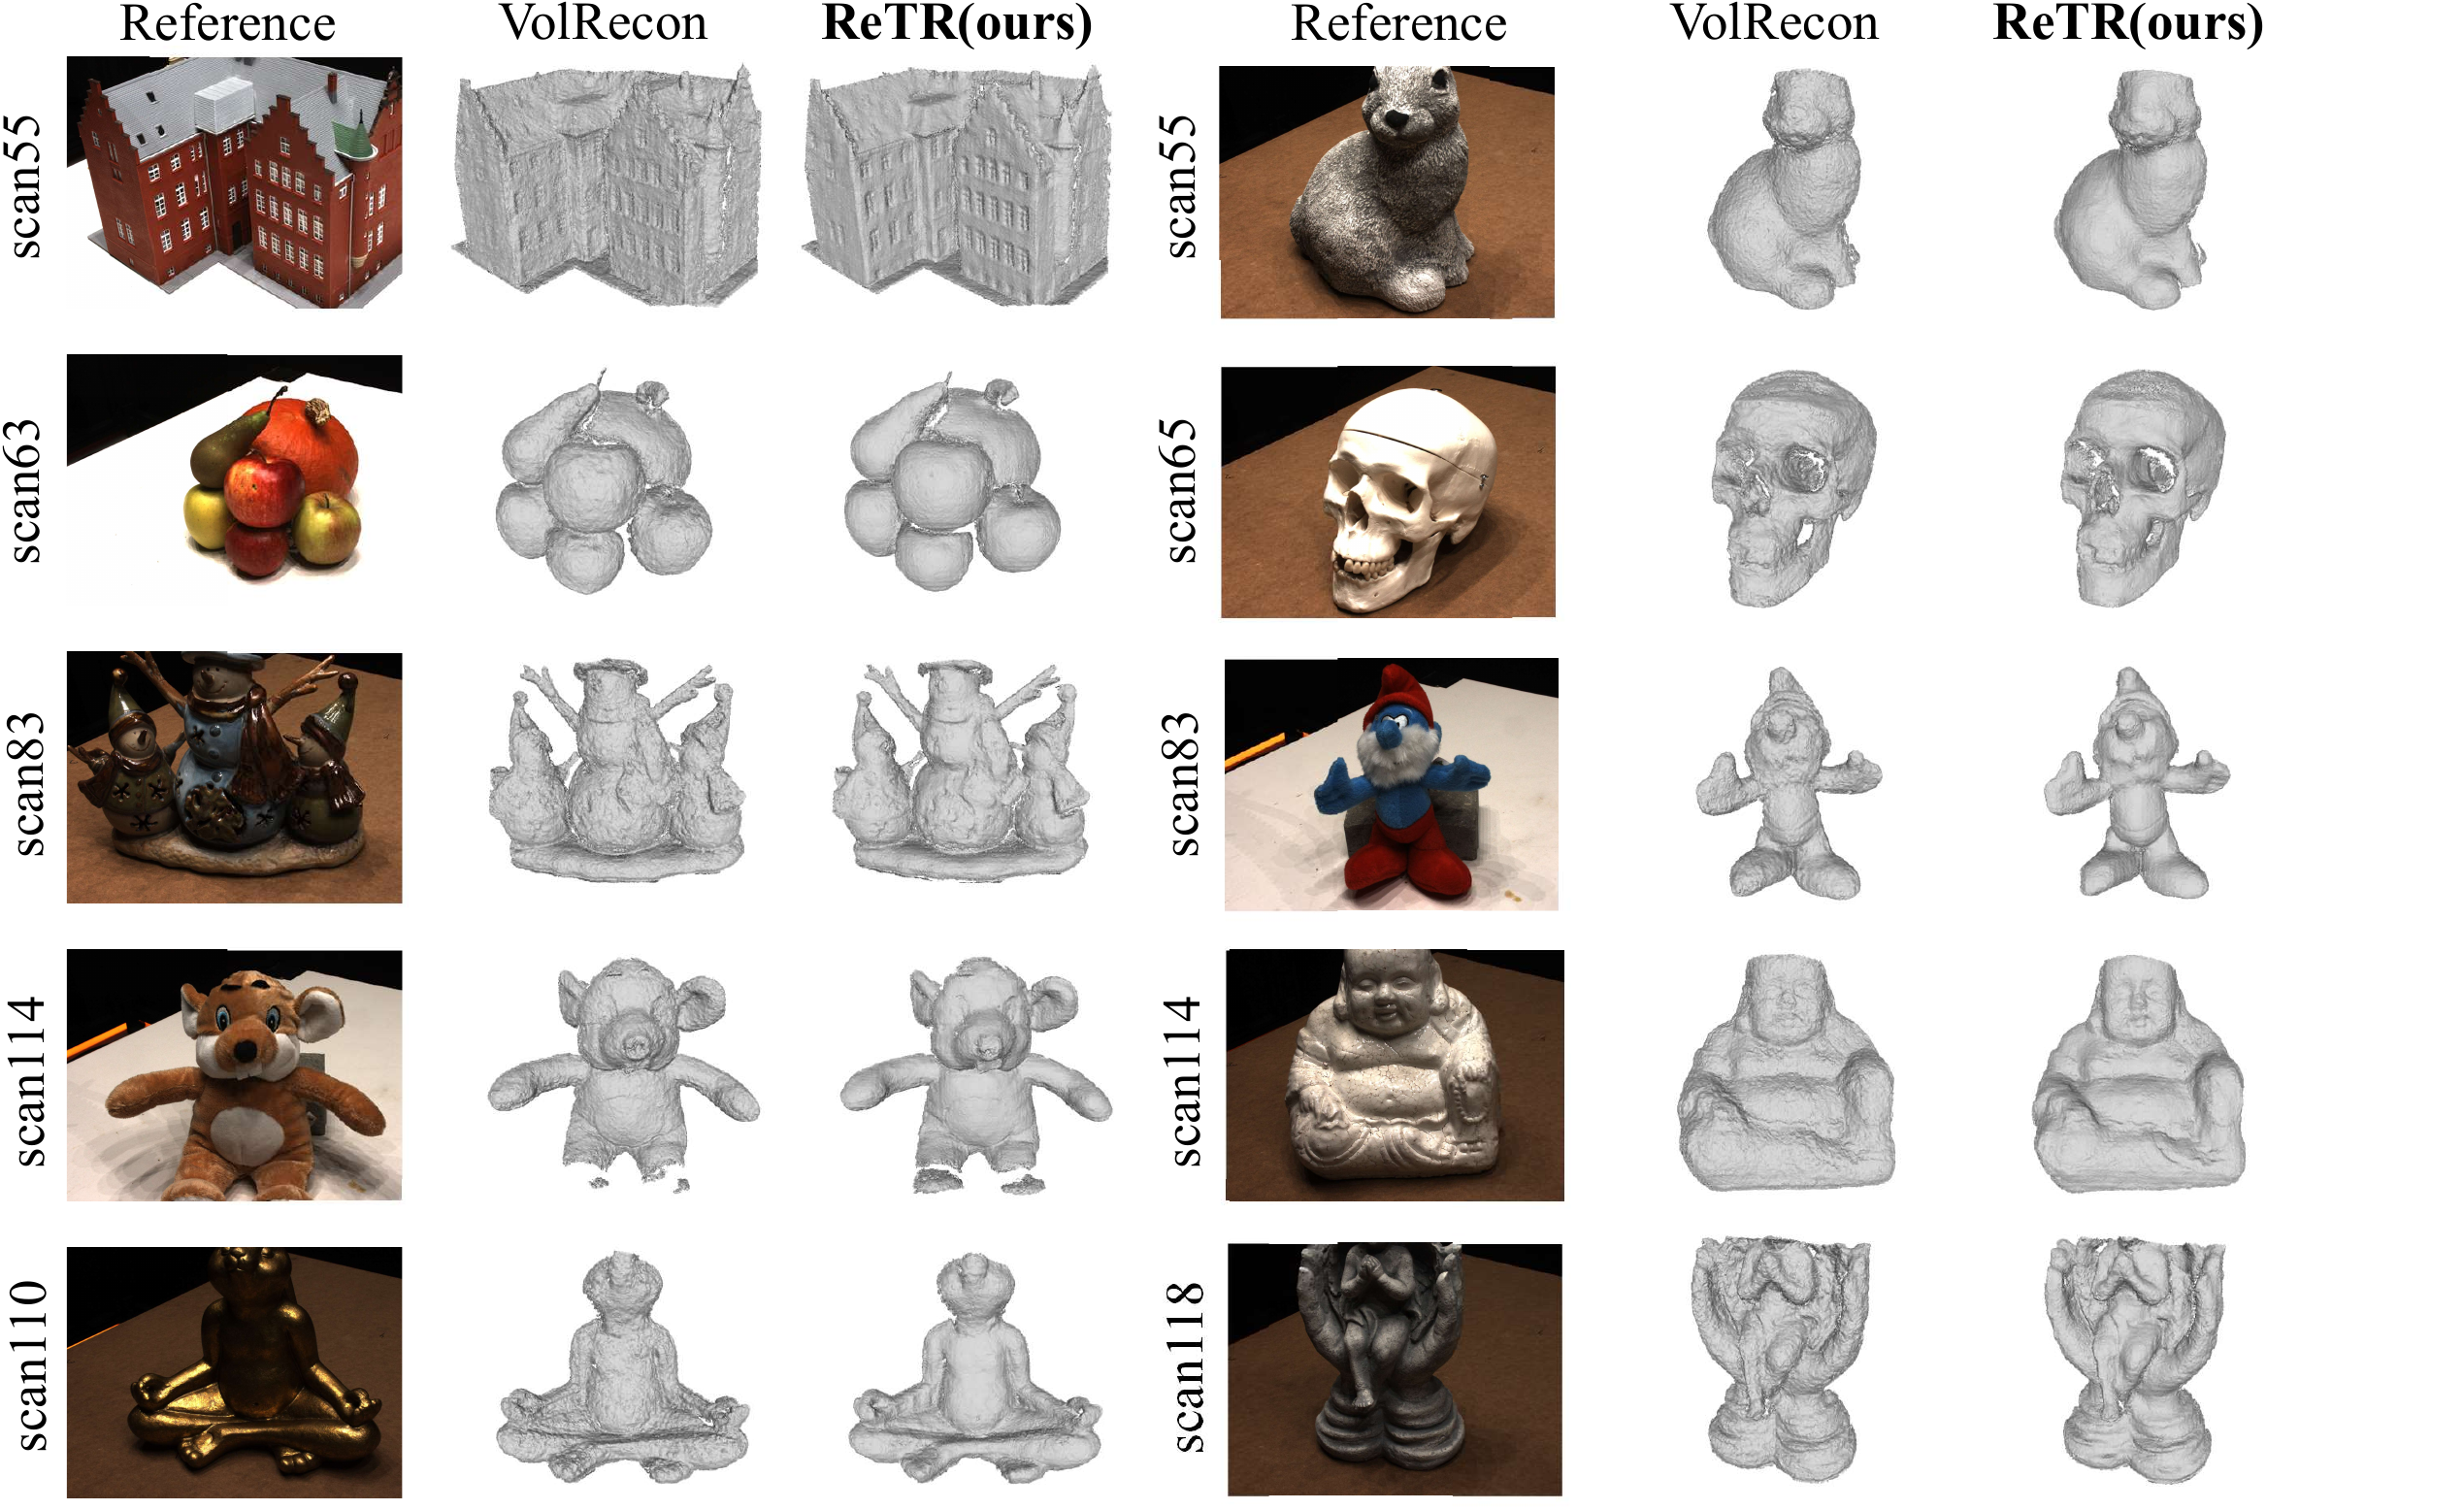}}
% \vspace{0.1cm}  
\caption{Comparison of VolRecon and ReTR in sparse view reconstruction with 3 input views.}
\label{fig:sprecon}
% \vspace{-0.8cm}  
\end{center}
\end{figure*}

\begin{figure*}[t]
%\vspace{-2em}
\begin{center}
\setlength{\abovecaptionskip}{0.cm}
\centerline{\includegraphics[width=1.0\textwidth]{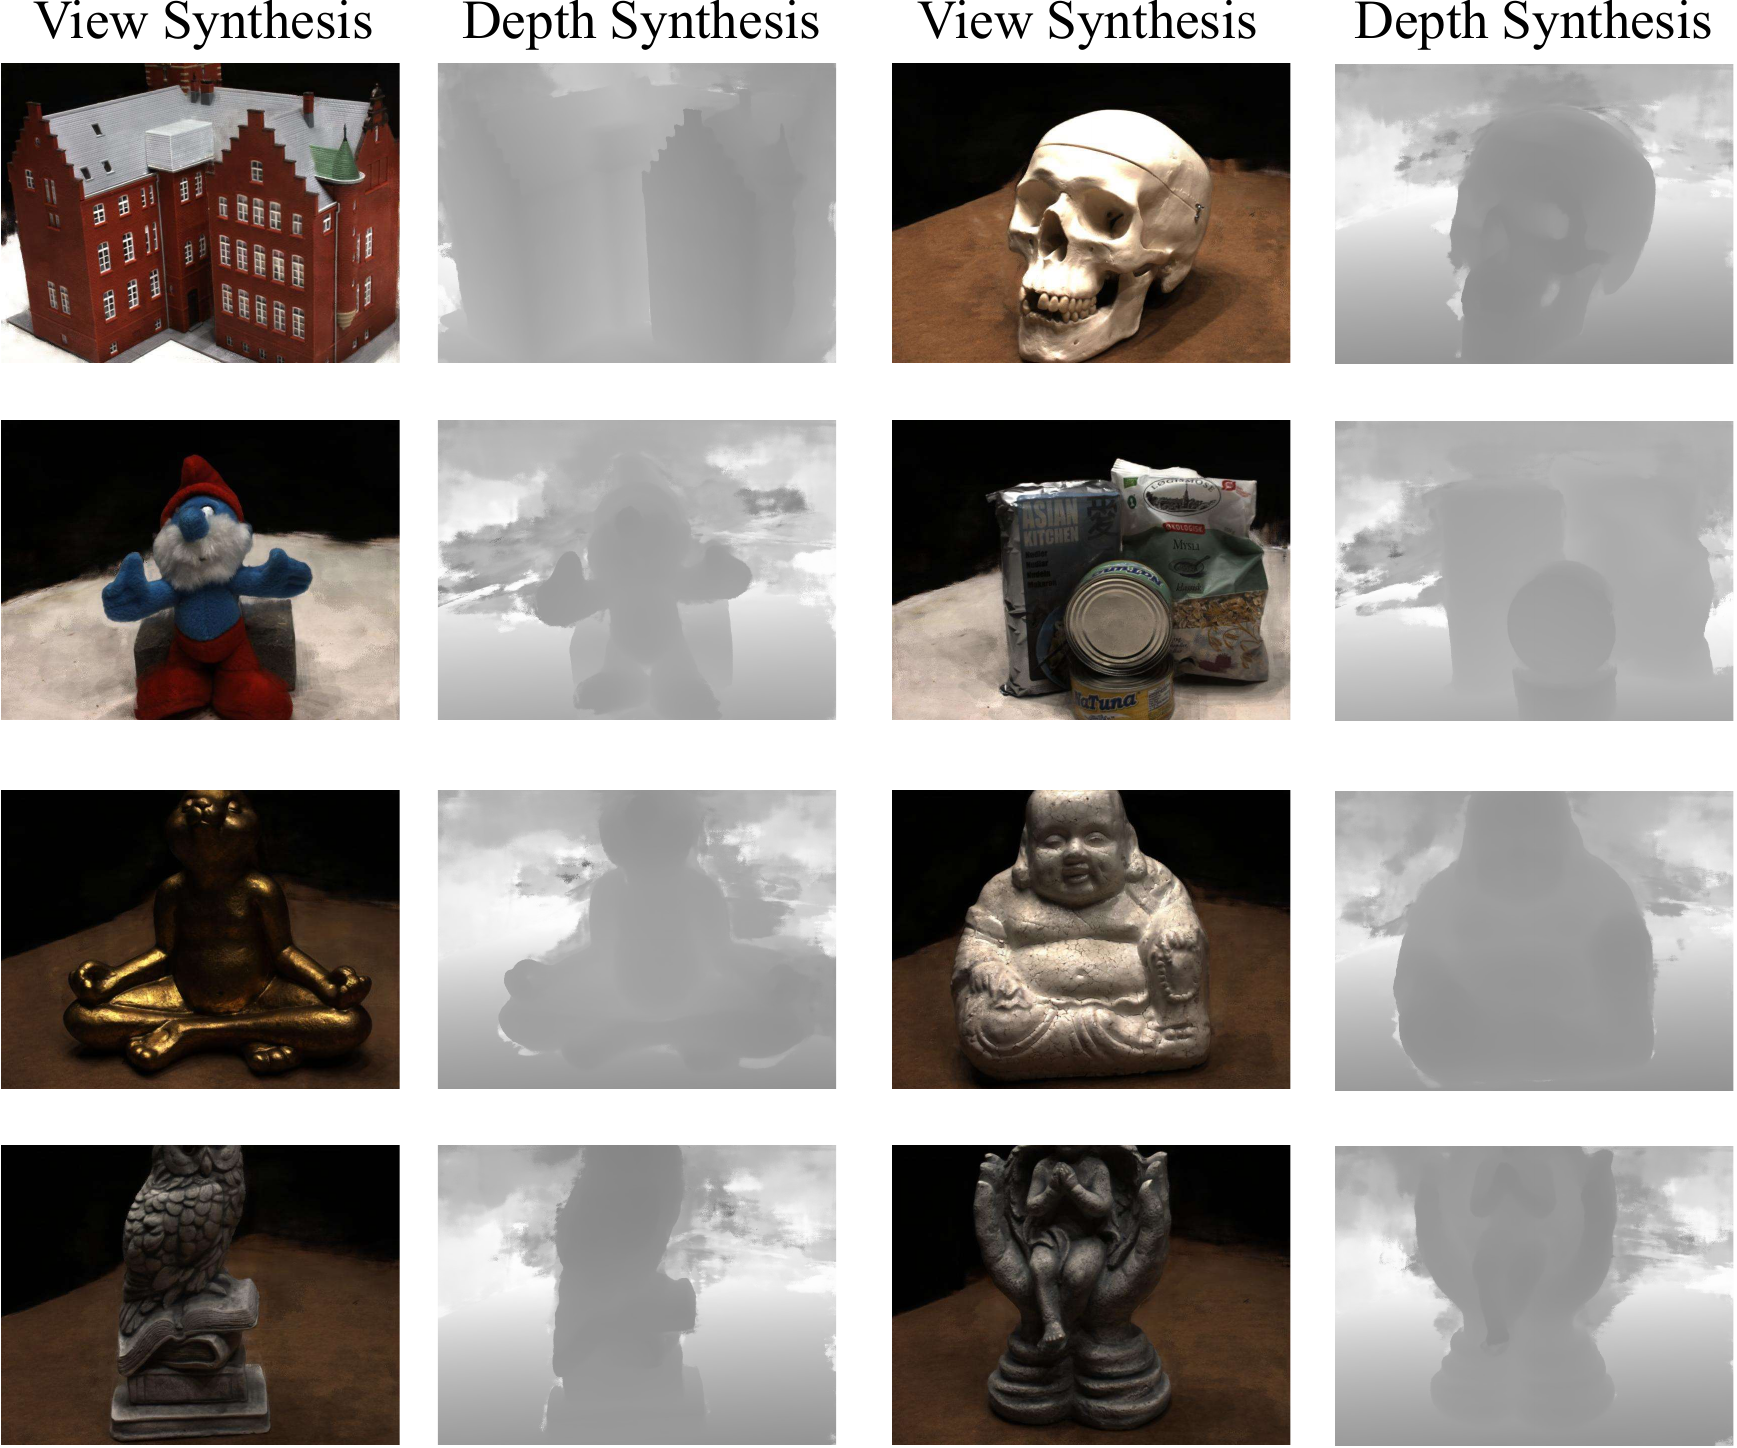}}
% \vspace{0.1cm}  
\caption{View synthesis and depth synthesis visualization of our proposed ReTR.}
\label{fig:synthesis}
% \vspace{-0.8cm}  
\end{center}
\end{figure*}
\begin{figure*}[t]
%\vspace{-2em}
\begin{center}
\setlength{\abovecaptionskip}{0.cm}
\centerline{\includegraphics[width=1.1\textwidth]{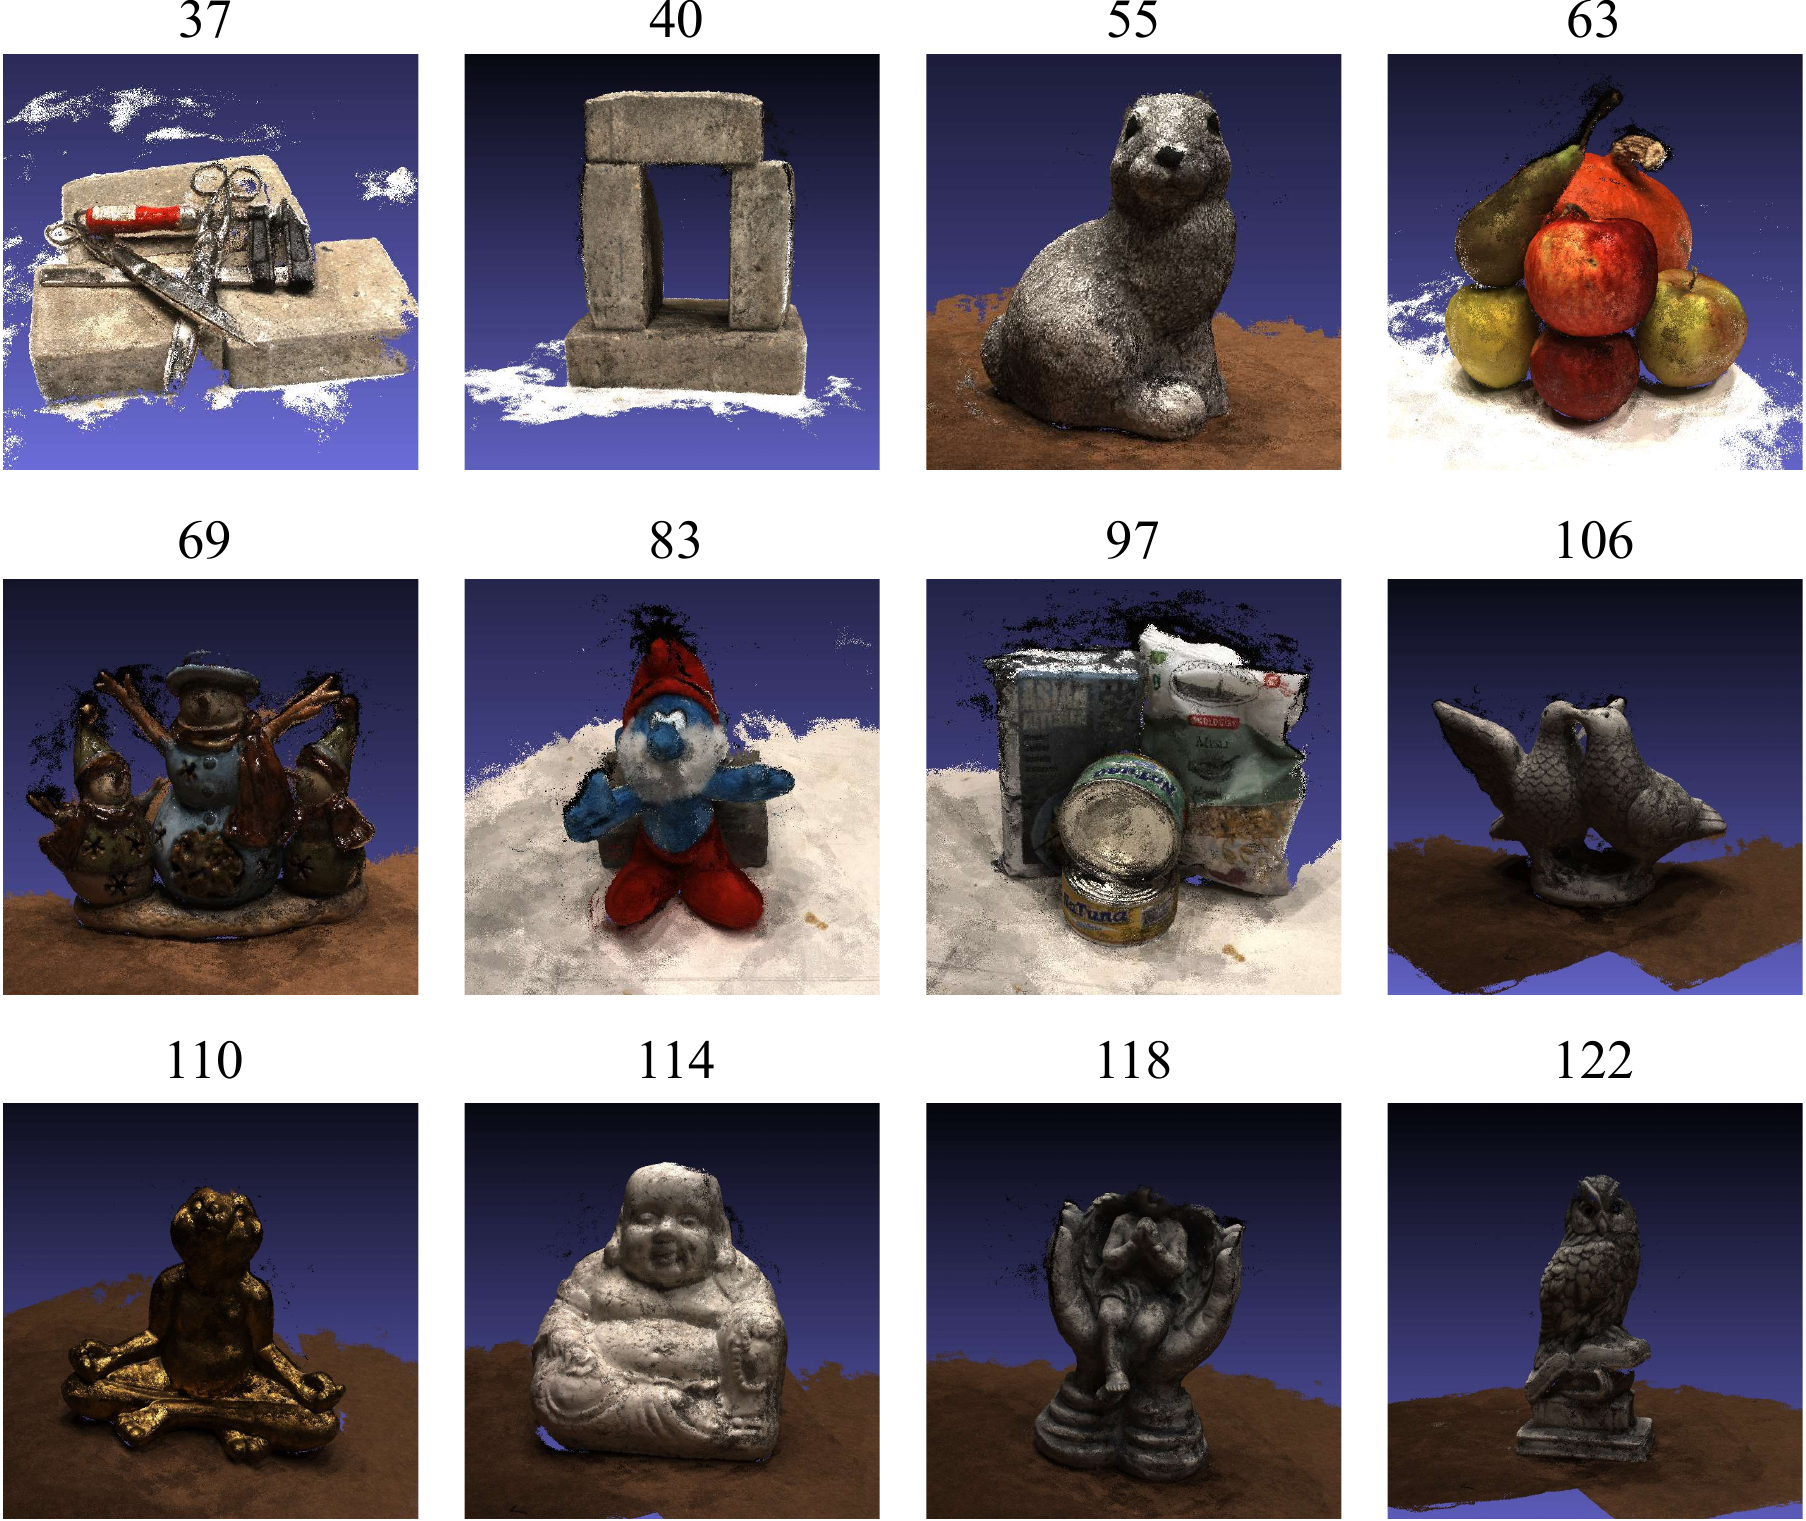}}
% \vspace{0.1cm}  
\caption{Visualization of full view generalization of a point cloud of our proposed ReTR.}
\label{fig:fullrec}
% \vspace{-0.8cm}  
\end{center}
\end{figure*}

\section{Limitations} 
Our method requires approximately 30 seconds to render a depth map and image with a resolution of $600\times800$. Similar to other rendering-based methods such as IBRNet~\cite{wang2021ibrnet}, VolRecon~\cite{ren2022volrecon}, and MVSNeRF~\cite{chen2021mvsnerf}, our approach has limitations in terms of efficiency.
While learning-based rendering offers enhanced capabilities, it does introduce additional training parameters compared to traditional volume rendering techniques. Stacking multiple layers of our model can improve performance; however, it also increases training time due to the larger model size.
It is important to strike a balance between achieving higher rendering quality and maintaining reasonable computational efficiency. Further research and optimization efforts can be explored to enhance the efficiency of our method, potentially through techniques such as model compression, parallelization, or hardware acceleration.
Acknowledging these limitations, we aim to provide a comprehensive understanding of the trade-offs between rendering quality, efficiency, and model complexity within our proposed framework.

\section{Broader Impacts}
The proposed ReTR framework not only enables accurate surface reconstruction through learnable rendering but also generates high-quality novel views. These capabilities open up possibilities for various downstream applications in fields such as virtual reality (VR), robotics, and view synthesis with geometry. While these applications offer numerous benefits, it is important to acknowledge that they also come with ethical considerations.
As authors of the ReTR framework, we are committed to promoting ethical practices and responsible development. We recognize the potential for misuse, such as generating content without consent, and we prioritize fair representation and responsible usage of the technology. We strive to adhere to ethical guidelines and contribute to the development of responsible AI practices. It is crucial to ensure that technological advancements are leveraged for the betterment of society while minimizing potential negative impacts.
By maintaining a focus on ethics, fairness, and responsible development, we aim to ensure that ReTR and its applications are aligned with the principles of responsible AI and contribute positively to the broader scientific community and society as a whole.
