# Supplementary material for: ReTR: Modeling Rendering Via Transformer for Generalizable Neural Surface Reconstruction
Source: arXiv:2305.18832 source file (2023-11-02)
Supplement: Supplementary file 3 [file appendix_sample_points.tex]

% Please add the following required packages to your document preamble:
% \usepackage{graphicx}
\begin{tabular}[]
\resizebox{\columnwidth}{!}{%
\begin{tabular}{cccccccccccccccc}\toprule
\multicolumn{1}{l}{Sample Points} &
  \multicolumn{1}{l}{scan 24} &
  \multicolumn{1}{l}{scan 37} &
  \multicolumn{1}{l}{scan 40} &
  \multicolumn{1}{l}{scan 55} &
  \multicolumn{1}{l}{scan 63} &
  \multicolumn{1}{l}{scan 65} &
  \multicolumn{1}{l}{scan 69} &
  \multicolumn{1}{l}{scan 83} &
  \multicolumn{1}{l}{scan 97} &
  \multicolumn{1}{l}{scan 105} &
  \multicolumn{1}{l}{scan 106} &
  \multicolumn{1}{l}{scan 110} &
  \multicolumn{1}{l}{scan 114} &
  \multicolumn{1}{l}{scan 118} &
  \multicolumn{1}{l}{scan 122} \\
16+16 & 1.09 & 2.49 & 1.51 & 1.09 & 1.62 & 1.64 & 0.97 & 1.35 & 1.43 & 1.05 & 1.21 & 0.77 & 0.72 & 1.27 & 1.28 \\
32+32 & 1.06 & 2.30 & 1.46 & 0.97 & 1.35 & 1.53 & 0.89 & 1.38 & 1.34 & 0.92 & 1.10 & 0.74 & 0.60 & 1.10 & 1.17 \\
64+0  & 1.11 & 2.39 & 1.43 & 1.06 & 1.36 & 1.62 & 0.94 & 1.28 & 1.31 & 0.91 & 1.12 & 0.78 & 0.64 & 1.18 & 1.20 \\
128+0 & 1.39 & 2.36 & 1.54 & 1.01 & 1.18 & 1.65 & 0.97 & 1.26 & 1.26 & 0.83 & 1.10 & 0.84 & 0.62 & 1.09 & 1.15
\end{tabular}%
}

\end{tabular}
